# Supplementary material for: DreamAvatar: Text-and-Shape Guided 3D Human Avatar Generation via Diffusion Models
Source: arXiv:2304.00916 source file (2023-11-30)
Supplement: Supplementary file 1 [file supplementary.pdf]

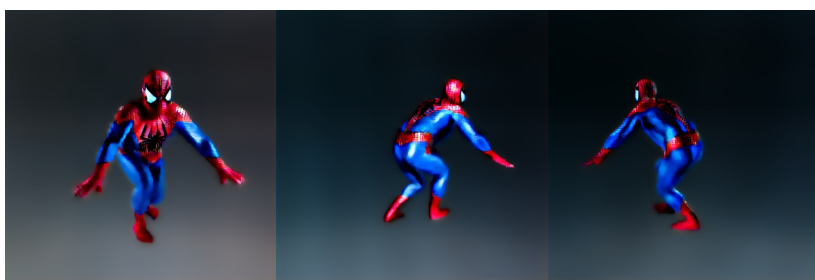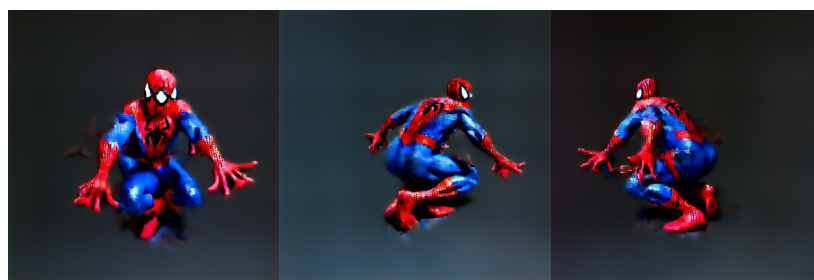

A standing Spiderman

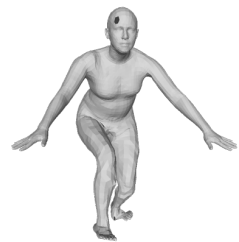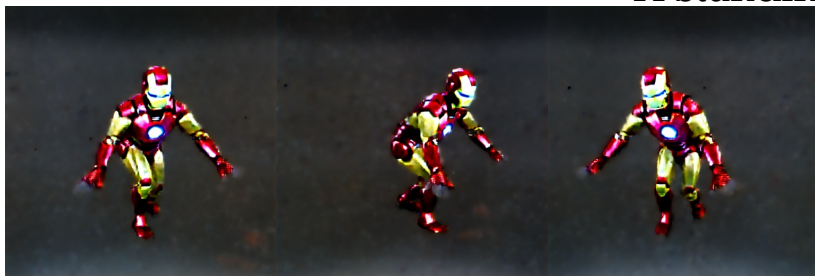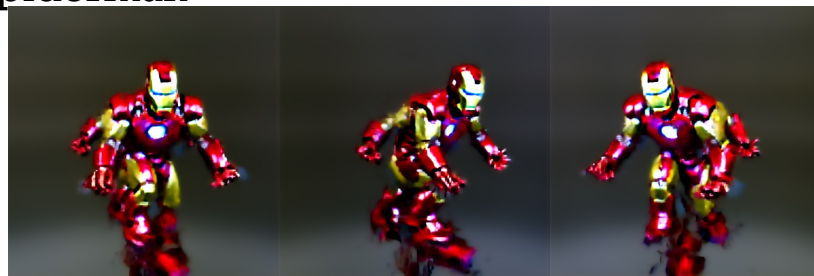

An iron man

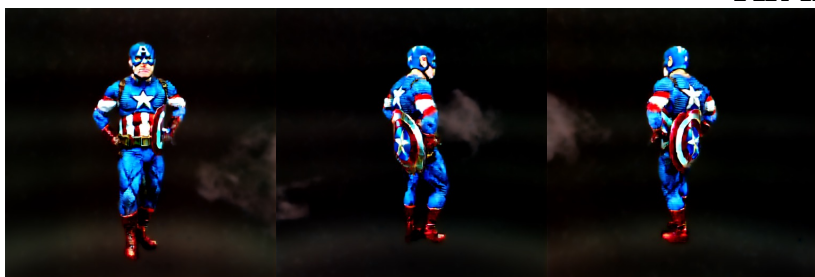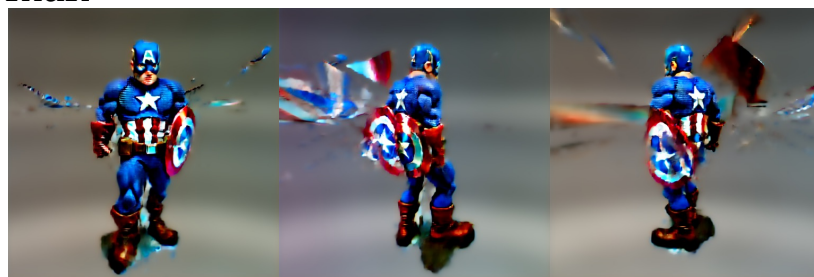

Captain America

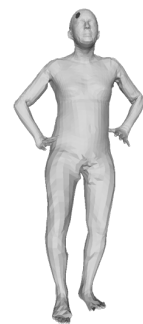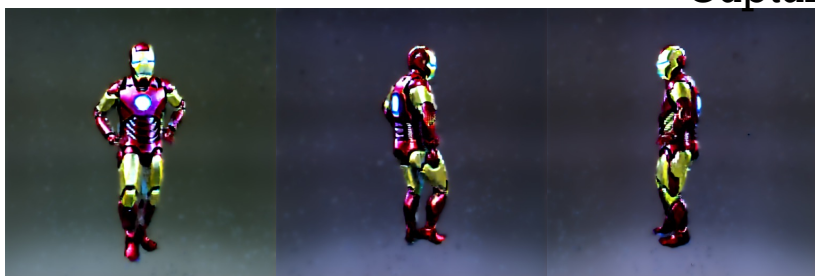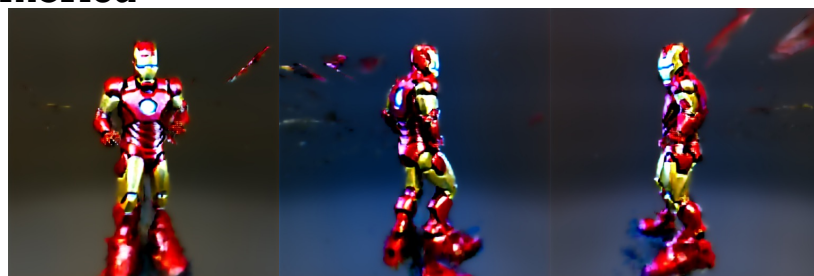

An iron man

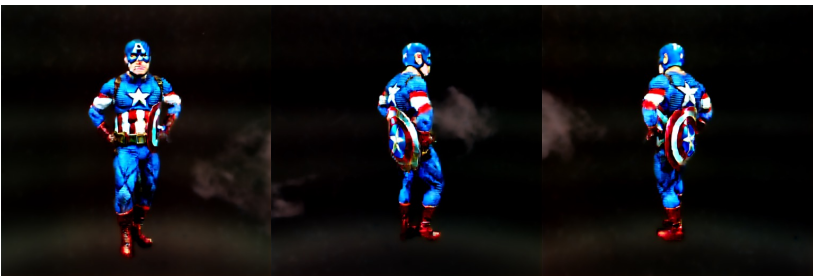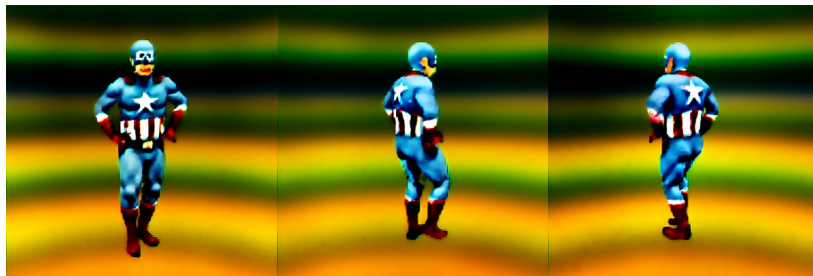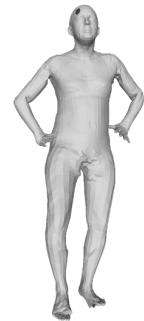

Captain America

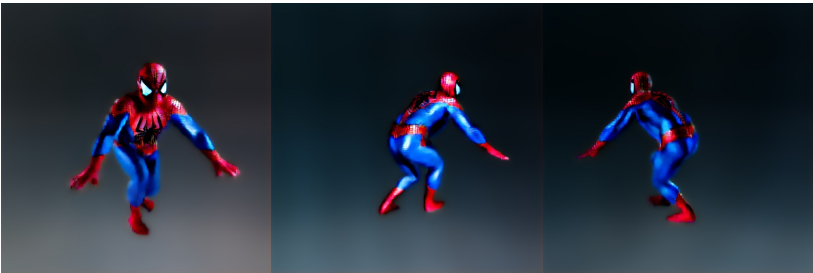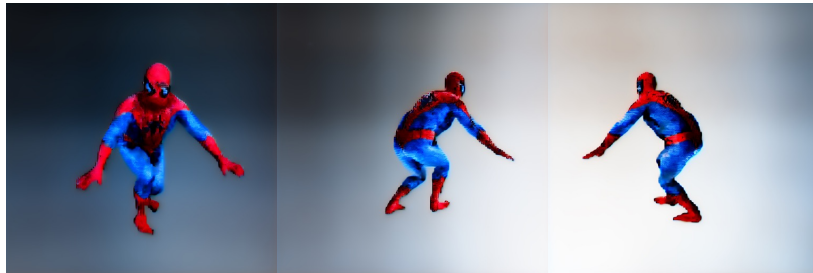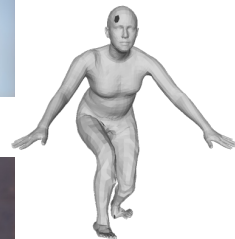

A standing Spiderman

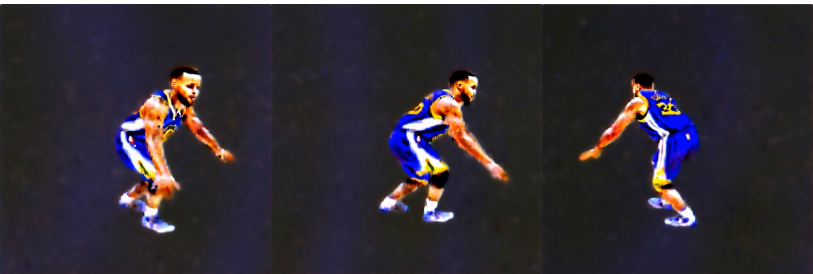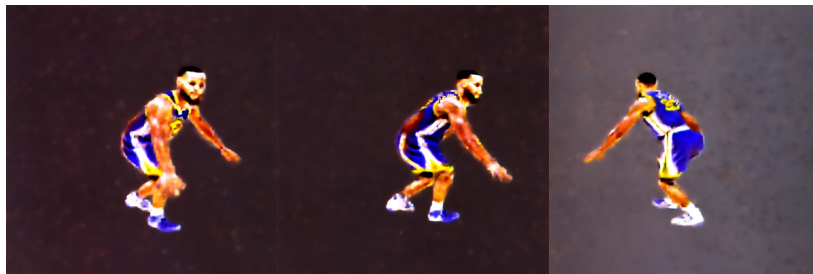

Stephen Curry, NBA player

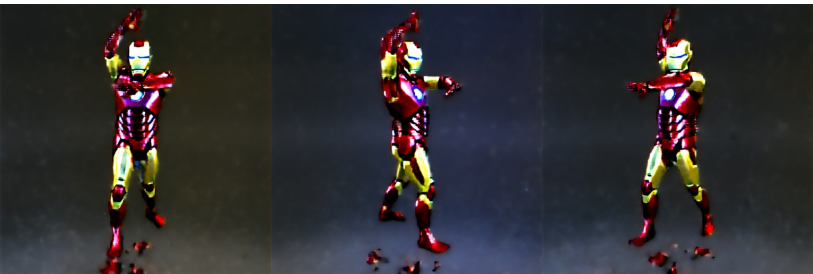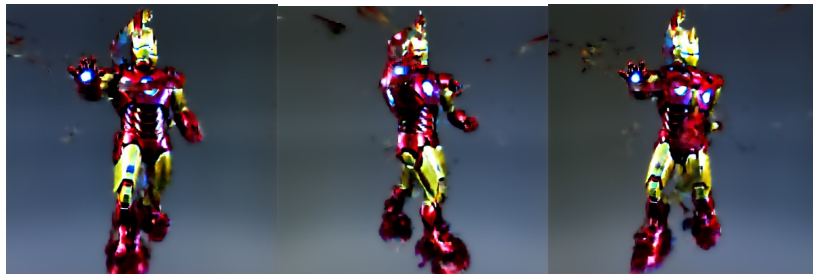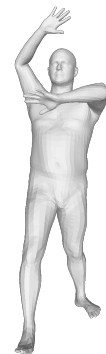

An iron man



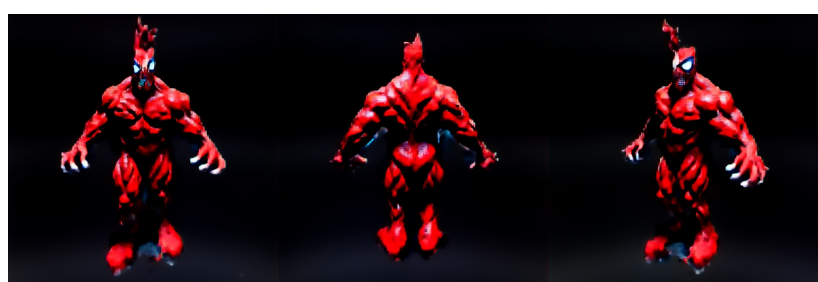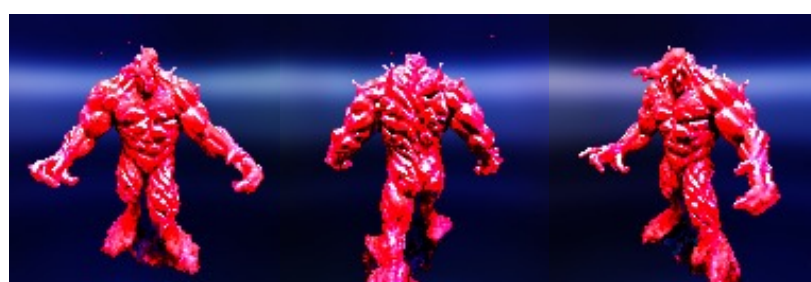

Carnage, marvel character

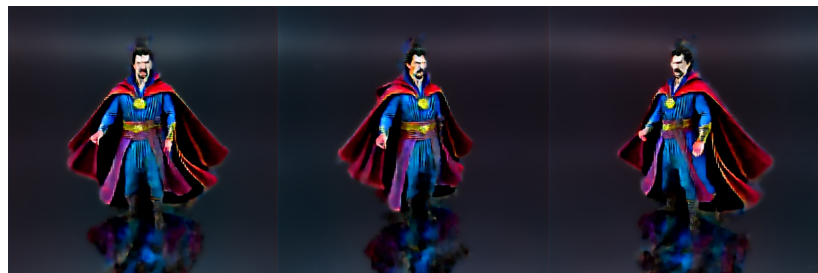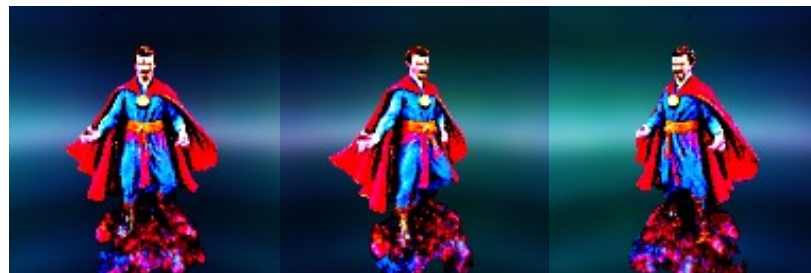

Doctor Strange

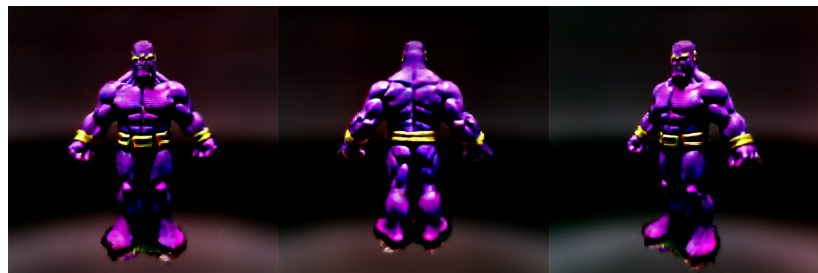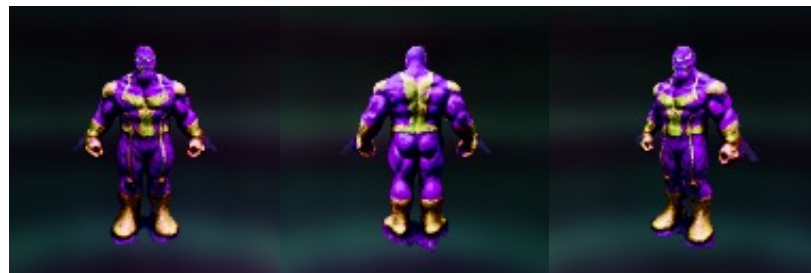

Thanos, marvel character

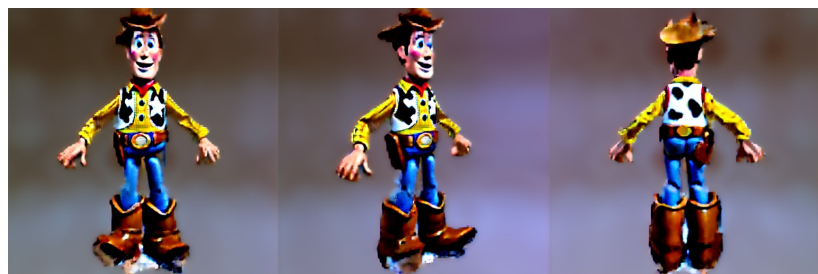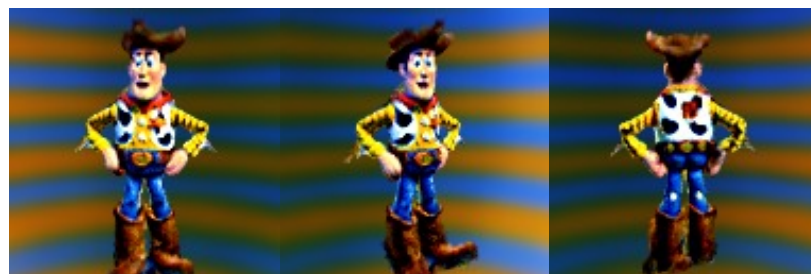

Woody in Toy Story

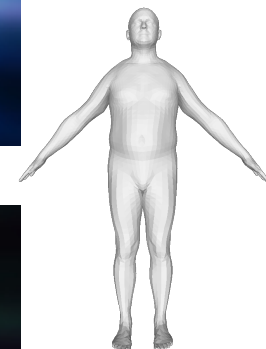

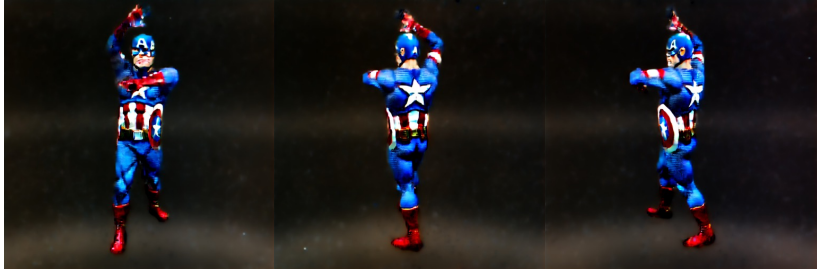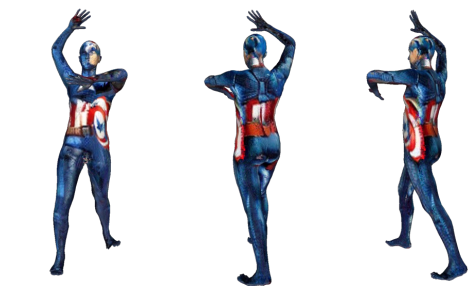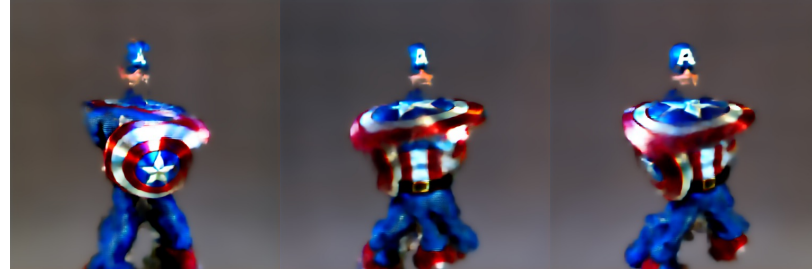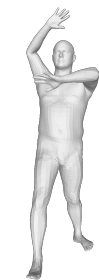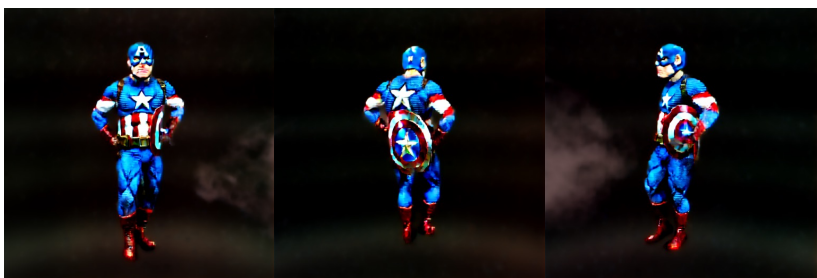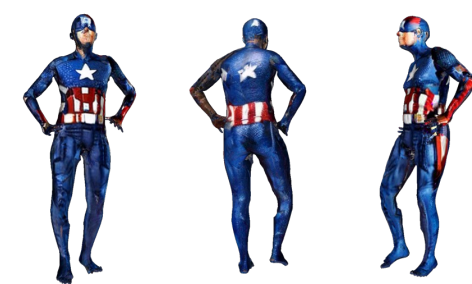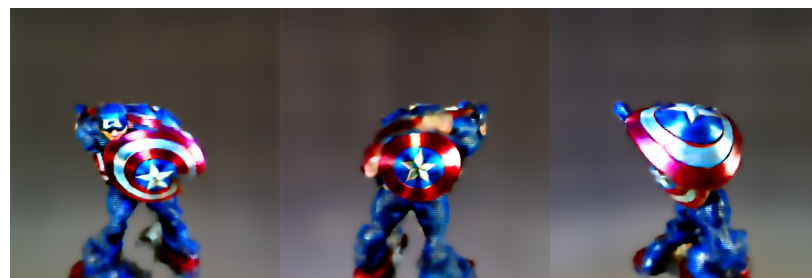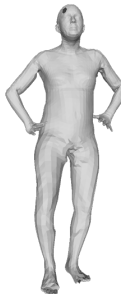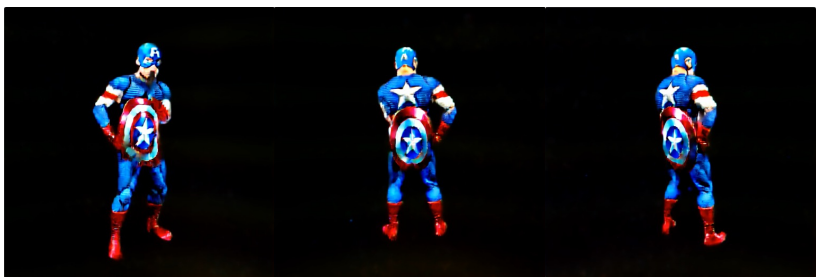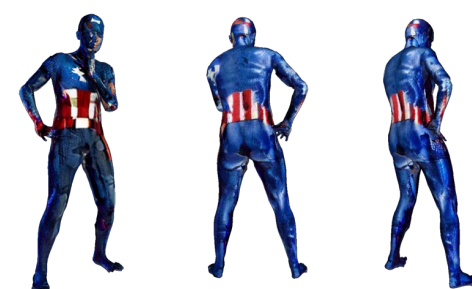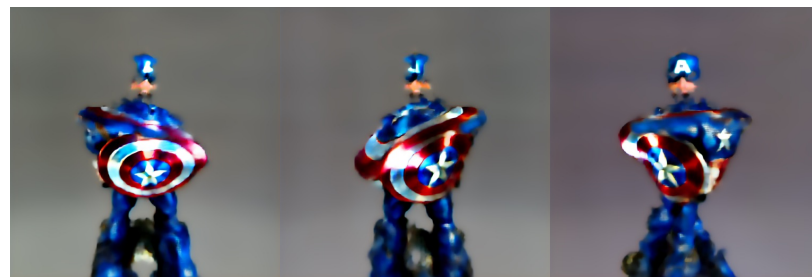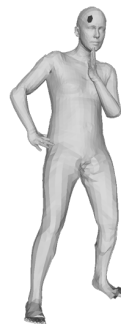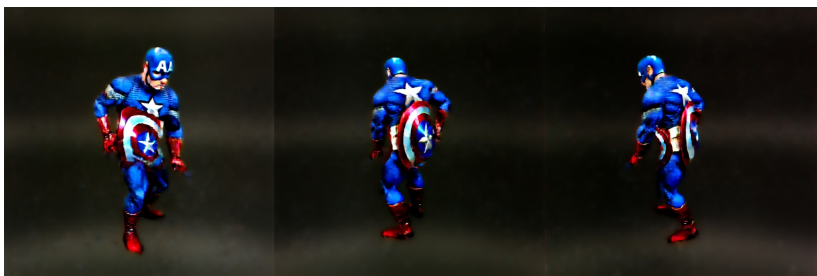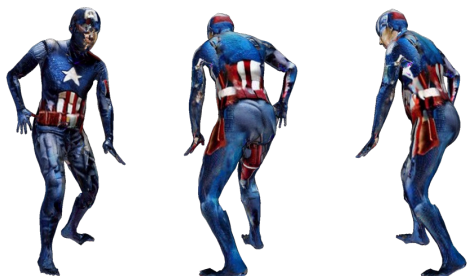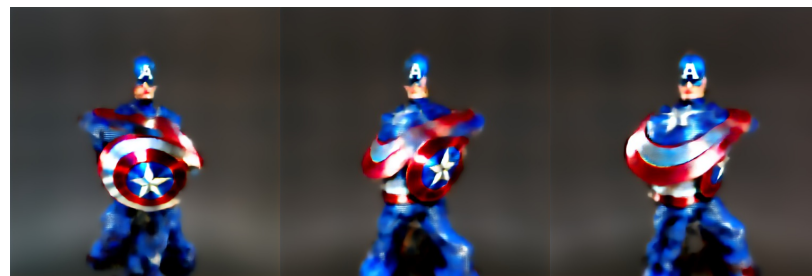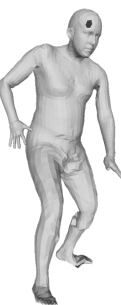

Ours

TEXTure

Latent-NeRF

Captain America



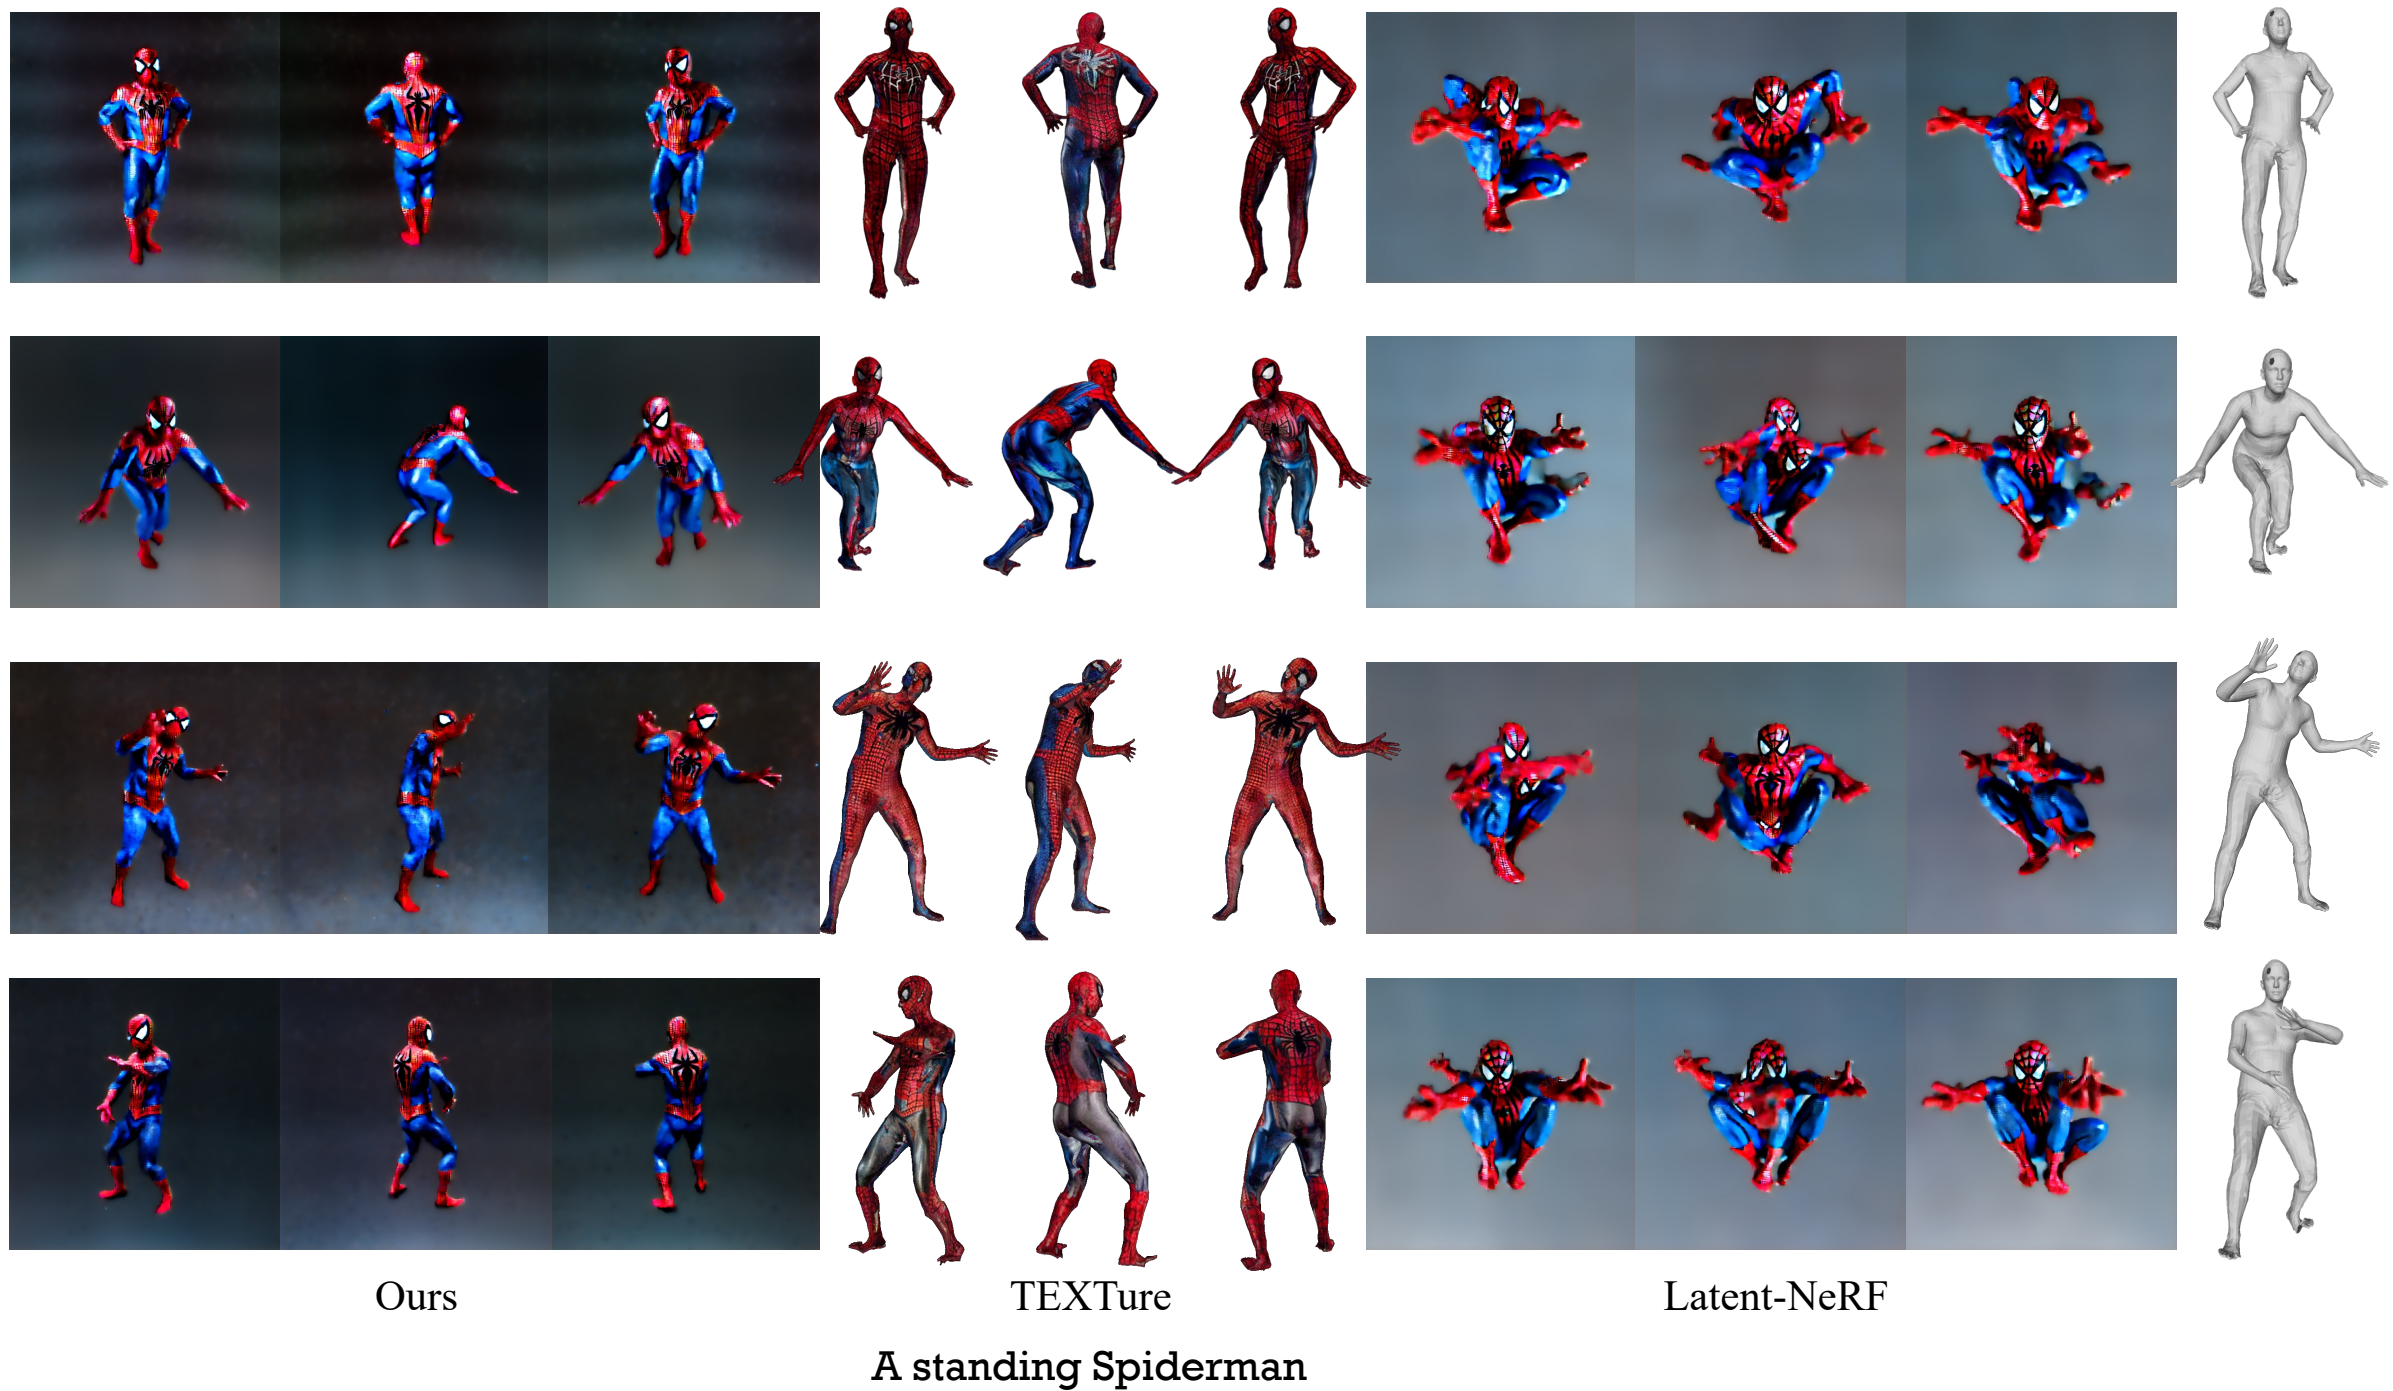

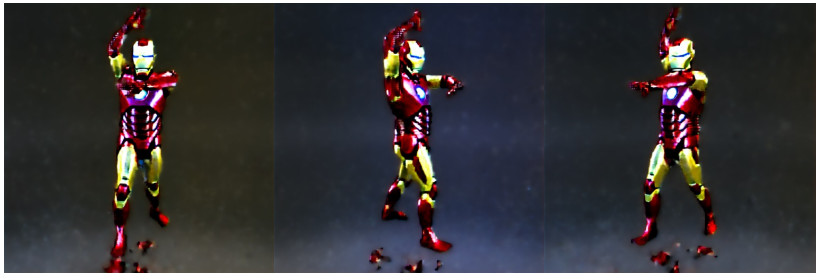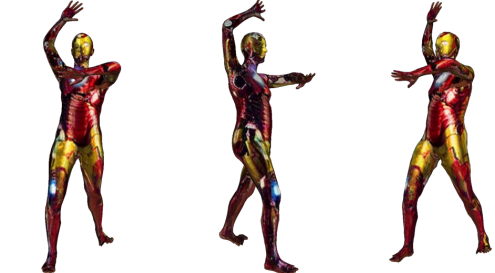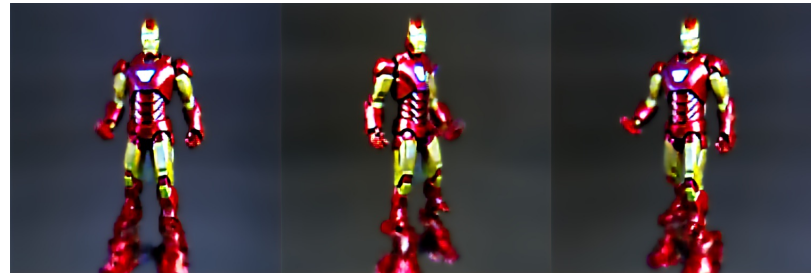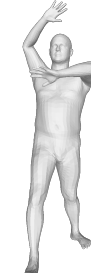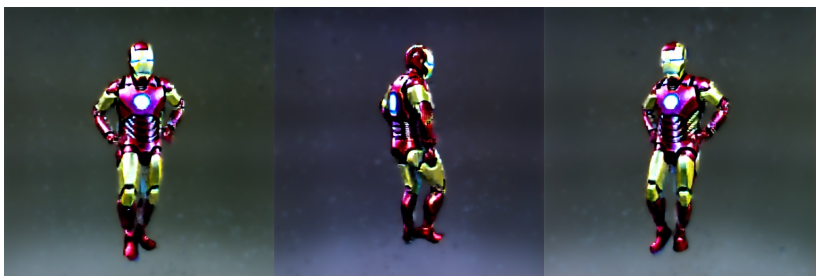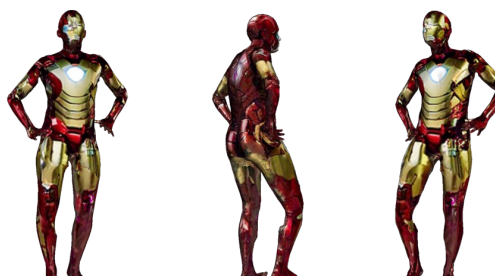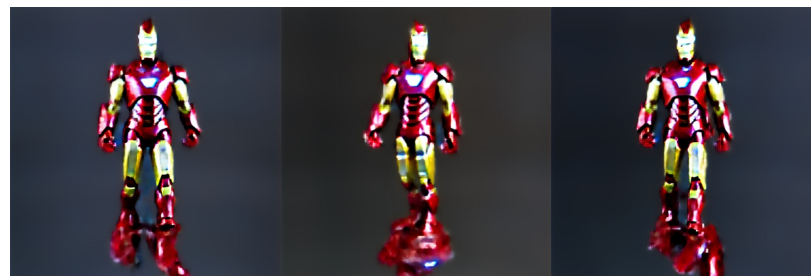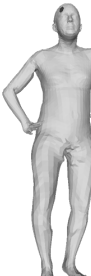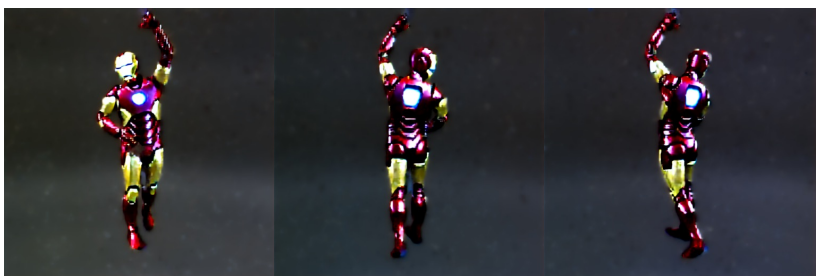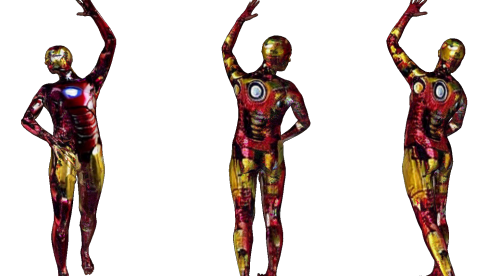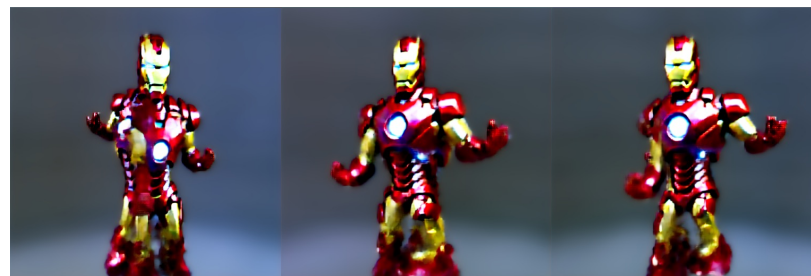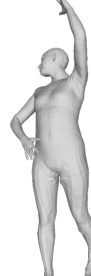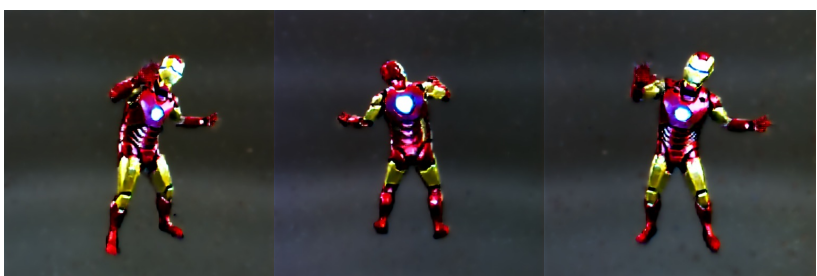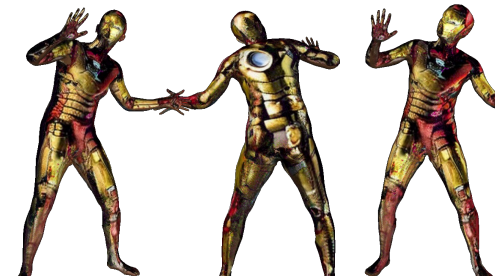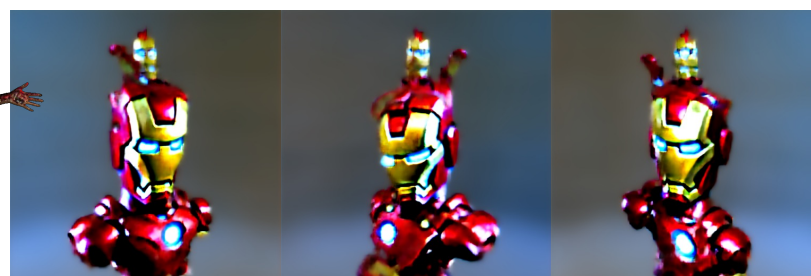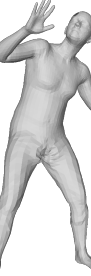

Ours

TEXTure

Latent-NeRF

An iron man
